# Supplementary material for: Edit3r: Instant 3D Scene Editing from Sparse Unposed Images
Source: arXiv:2512.25071 source file (2025-12-31)
Supplement: Supplementary file 1 [file X_suppl.tex]

\clearpage
\setcounter{page}{1}

\twocolumn[{% 
\renewcommand\twocolumn[1][]{#1}% 
\maketitlesupplementary
\begin{center} 
% \vspace{-0.2in}
\vspace{8mm}
\centering 
\includegraphics[width=\textwidth]{fig/Supp_pipeline.pdf}
    \captionsetup{width=\linewidth}
    \captionof{figure}{\textbf{\ourmethod} Backbone pipeline.}
    \label{fig:edit3r-arch}
    \vspace{4mm}
\end{center}
}]

\section{Method \& Architecture Details}
\label{sec:arch}
\subsection{Detailed Structure}

Figure~\ref{fig:edit3r-arch} illustrates the network architecture of {\ourmethod}.
Our model is built upon the pose-free large reconstruction model NoPoSplat~\cite{noposplat} and follows the same encoder--decoder--head design, while adapting it to asymmetric edited inputs for 3D scene editing.

\paragraph{Inputs and tokenization.}
Given two unposed RGB views and their camera intrinsics
\(\{(I'_0, k_0), (I_1, k_1)\}\),
where \(I'_0\) is the recolored (edited) reference view and \(I_1\) is an unedited auxiliary view,
our goal is to predict a single canonical 3D Gaussian scene that represents the edited content.
Each image is resized and patchified, and a Vision Transformer (ViT)~\cite{vit} encoder operates on the resulting sequence of image tokens.
Following NoPoSplat~\cite{noposplat}, we embed the intrinsics \(k_v\) of each view with a small MLP
\(\phi: \mathbb{R}^d \rightarrow \mathbb{R}^D\) and append the resulting \emph{intrinsics token} to the image tokens:
\begin{equation*}
    z_v = \big[\,\text{img\_tokens}(I_v) \oplus \phi(k_v)\,\big],
\end{equation*}
This intrinsic-token strategy improves scale stability and removes the need for pose supervision, as observed in~\cite{noposplat}.

\paragraph{Shared ViT encoder.}
The two views are processed independently by a shared-weight ViT encoder.
For each view \(v\), the encoder produces a sequence of latent tokens
\(f_v\) at a constant spatial resolution (downsampled with respect to the input image).
At this stage, the views do not interact; each \(f_v\) encodes high-level appearance and coarse geometry for its corresponding image.

\paragraph{Multi-view ViT decoders with cross-attention.}
To fuse information across views, {\ourmethod} employs two identical ViT decoders, one per view, that communicate via cross-attention (Fig.~\ref{fig:edit3r-arch}).
Each decoder takes the encoder features \(f_v\) as input and consists of a stack of transformer blocks.
Within each block, self-attention is applied to tokens from a single view, while a cross-attention layer lets tokens from one view attend to tokens from the other view.
In the two-view setting, this yields two decoder branches with shared parameters, where features for \(I'_0\) and \(I_1\) are refined jointly.
This design allows the model to resolve occlusions and reconcile the potentially inconsistent appearance between the edited reference view and the unedited auxiliary view, while still preserving view-specific details.

\paragraph{DPT-based Gaussian prediction heads.}
From the fused decoder features, {\ourmethod} predicts per-pixel Gaussian parameters using two dense prediction heads per view, both based on the DPT architecture~\cite{dust3r}. For view \(v\), let \(f_{fused-v}\) denote the output of the ViT decoder.

\begin{itemize}
    \item \textbf{Center head.}
    The \emph{center head} takes only \(f_{fused-v}\) as input and upsamples it via a DPT-style decoder to full image resolution.
    It regresses a 3D center \(\boldsymbol{\mu} \in \mathbb{R}^3\) for each pixel, yielding a dense field of Gaussian centers in a canonical world frame.

    \item \textbf{Parameter head.}
    The \emph{parameter head} predicts the remaining Gaussian attributes.
    It receives both the decoder features and a high-resolution RGB shortcut from the corresponding input image:
    \begin{equation}
        \mathbf{H}_v = \mathrm{concat}\!\big(f_{fused-v}, \mathrm{RGB\_feat}(I_v^{\mathrm{RGB}})\big),
    \end{equation}
    where \(I_v^{\mathrm{RGB}}\) is \(I'_0\) for the edited reference branch and \(I_1\) for the auxiliary branch.
    A DPT decoder processes \(\mathbf{H}_v\) and predicts opacity \(\alpha\), anisotropic covariance parameters (orientation and scale), and low-order spherical-harmonic color coefficients \(c\) for each pixel.
    The RGB shortcut compensates for the lower spatial resolution of ViT features and is crucial for recovering fine-grained textures and edges, as also reported in~\cite{noposplat}.
\end{itemize}

For each pixel in each view we thus obtain a Gaussian
\(({\mu}_j, {\Sigma}_j, \alpha_j, c_j)\).
All Gaussians are expressed directly in the canonical coordinate system and do not require any explicit pose estimation or local-to-global transformation.

\paragraph{Canonical-space fusion and rendering.}
The Gaussian primitives from the two branches are concatenated to form a single set
\(\mathcal{G} = \{(\mu_j, \Sigma_j, \alpha_j, c_j)\}\)
representing the edited 3D scene.
We render \(\mathcal{G}\) using standard 3D Gaussian splatting to obtain supervision views during training (recolored targets) and novel edited views at inference time.
Because the two decoder branches share weights and interact via cross-attention, {\ourmethod} learns to fuse the edited reference view and the unedited auxiliary view into a coherent 3D representation, even when the 2D edits are view-inconsistent.

\paragraph{Differences from NoPoSplat.}
Architecturally, {\ourmethod} reuses the NoPoSplat backbone (ViT encoder, multi-view ViT decoder with cross-attention, and DPT center/parameter heads) but changes the input configuration and training objectives.
The encoder--decoder now receives an \emph{asymmetric} pair of images \((I'_0, I_1)\), and the RGB shortcuts for the parameter heads are taken from the edited and unedited images, respectively.
Combined with our SAM2-based recoloring, asymmetric input scheme, and 3D regularization losses, this architecture enables {\ourmethod} to map view-inconsistent 2D edits to a single, view-consistent set of 3D Gaussians while retaining the fast, feed-forward inference of the original pose-free reconstructor.

\subsection{Training Loss Detail}
During training, our model is optimized with a combination of 2D appearance losses and 3D geometric regularizers, applied to every supervision view. Given the rendered prediction $\hat{I}_v$ for view $v$ and its corresponding ground-truth image $I_v$, we minimize a weighted sum of a CLIP-based semantic loss, a perceptual LPIPS loss, and a low-frequency MSE loss over all views, together with two 3D losses that regularize the predicted Gaussian scene structure. Formally, the total loss can be written as
\begin{equation*}
\begin{split}
\mathcal{L}_{\text{total}}
= \sum_{v} \Big(
\lambda_{\text{CLIP}} \mathcal{L}_{\text{CLIP}}(\hat{I}_v, I_v)
+ \lambda_{\text{LPIPS}} \mathcal{L}_{\text{LPIPS}}(\hat{I}_v, I_v)\\
+ \lambda_{\text{MSE}} \mathcal{L}_{\text{MSE}}(\hat{I}_v, I_v)
\Big)
+ \lambda_{\text{center}} \mathcal{L}_{\text{center}}
+ \lambda_{\text{geom}} \mathcal{L}_{\text{geom}}.
\end{split}
\end{equation*}
As mentioned in the main paper, the scalar weights $\lambda_{\cdot}$ correspond to the configuration weights of each loss module, with $\lambda_{\text{CLIP}} = 0.5$, $\lambda_{\text{LPIPS}} = 0.8$, $\lambda_{\text{MSE}} = 1.0$, $\lambda_{\text{center}} = 0.01$, and $\lambda_{\text{geom}} = 0.03$.

\begin{figure*}[t]
    \centering
    \includegraphics[width=\textwidth]{fig/Supp_sam.pdf}
    \caption{\textbf{SAM2 segmentation detailed pipeline.}}
    \label{fig:supp_sam}
\end{figure*}

\subsection{SAM2 Configuration and Usage}
\label{sec:sam2_supp}

We adopt the official SAM2 implementation with the \texttt{sam2.1\_hiera\_small} checkpoint and use it in two stages: (i) object discovery on the first frame, and (ii) mask propagation over the entire video. Concretely, we instantiate a \texttt{SAM2AutomaticMaskGenerator} with the following hyperparameters:
\begin{itemize}
    \item \texttt{points\_per\_side} $= 32$,
    \item \texttt{pred\_iou\_thresh} $= 0.7$,
    \item \texttt{stability\_score\_thresh} $= 0.92$,
    \item \texttt{crop\_n\_layers} $= 1$,
    \item \texttt{crop\_n\_points\_downscale\_factor} $= 2$,
    \item \texttt{min\_mask\_region\_area} $= 100$.
\end{itemize}
On the first frame of each sequence, the automatic mask generator proposes candidate regions. We then apply the deterministic multi-criterion filter defined in the main paper: a mask is kept only if (i) its area $A$ is at least
$A_{\min} = 400$ pixels, (ii) its stability score $s$ satisfies
$s \geq s_{\min} = 0.92$, (iii) its predicted IoU $q$ satisfies
$q \geq q_{\min} = 0.7$, (iv) the aspect ratio of its bounding box
$r = w/h$ lies in $[r_{\min}, r_{\max}] = [0.1, 10]$ (to avoid
extremely thin or flat regions), and (v) its bounding box has at least
$m_{\text{edge}} = 10$ pixels of margin to the image boundary on all sides.
The remaining instances are sorted by area, and we retain at most $N_{\max} = 20$ objects per sequence.

For temporal tracking, we use the SAM2 video predictor. We first initialize an internal inference state on the extracted frame sequence and then add each selected mask on the first frame as a separate object ID. We run the built-in \texttt{propagate\_in\_video} routine to obtain per-frame mask logits for each object; logits are binarized at zero to produce final foreground masks. To suppress identity drift, we compare the set of active object IDs in each frame to that of the most recently accepted frame and discard a frame if the size of their intersection is smaller than $0.5$ times the larger of the two set cardinalities. Such frames are excluded from subsequent processing (including our recoloring and supervision stages).

An example of this pipeline is visualized in Fig.~\ref{fig:supp_sam}. For each video, SAM2 first performs object-level segmentation on the initial frame and returns up to 20 candidate masks (three of which are shown). These selected masks are then propagated to subsequent frames by the video predictor, which maintains object identities over time and yields temporally consistent foreground masks. Applying our recoloring procedure to each frame based on these propagated masks produces coherent multi-frame edits.

\subsection{3D Regularization}
\begin{figure}
\scriptsize
    \centering
    \includegraphics[width=\linewidth]{fig/Supp_3Dloss.pdf}
    \caption{\textbf{Examples of training results without 3D constraints.}}
    \label{fig:supp_3dloss}
    \vspace{-4mm}
\end{figure}

\paragraph{Motivation.}
Text-driven 2D scene editing inevitably perturbs the appearance and depth cues of the input views in a view-dependent way. In our setting, the underlying scene geometry is expected to remain close to the original reconstruction, but the edited images no longer follow a single, globally consistent depth field. As a consequence, if we only optimize 2D reconstruction losses, the model can fit the edited supervision by sliding Gaussian primitives along the viewing rays: the rendered images still match the edited inputs, but the predicted Gaussian centers drift in depth and the reconstructed surfaces become distorted.
As shown in Fig.\ref{fig:supp_3dloss}(a), when training with 2D losses only, the Gaussians predicted from the two views yield human heads of noticeably different sizes: the Gaussian centers in the edited view are pulled towards the camera in an attempt to cover the content in view2, while the centers in view2, being largely occluded, become unconstrained and drift backwards.
%如图（a）部分所示，在只加2D loss训练的情况下，两个view预测的两个gaussian之间出现了不同大小的人头，gaussian center会出现往镜头方向移动的情况，试图覆盖掉view2，而view2因为被覆盖住了，gaussian center的位置就不受控制了,往后扩大

This issue is further exacerbated by our asymmetric input design, where the edited reference view and the unedited auxiliary view undergo different amounts and patterns of appearance change. The network then tends to explain each view with a different depth configuration, which leads to view-dependent ``layering'' and misalignment of the 3D Gaussians reconstructed from different views. In practice, we observe that, without additional 3D constraints, the same physical surface may be represented by different depth layers in the two views. 
As shown in Fig.\ref{fig:supp_3dloss}(b), training with 2D losses only also causes a layered structure between the Gaussians from view1 and view2, where the Gaussians of view1 are consistently pushed forward along the viewing direction in an attempt to cover those from view2.
%如图（b）所示，在只加2D loss训练的情况下，导致的另一个结果是view1的gaussian和view2的gaussian出现分层的情况，view1会尽量往前把view2覆盖住

\paragraph{3D Loss Design.}
To prevent such degenerate solutions, we introduce two complementary 3D losses. First, we apply a depth/center regularization loss that anchors the edited Gaussians to the reference centers predicted by a frozen LRM on the unedited images. This term constrains the optimization to stay close to the original 3D geometry and avoids large depth shifts caused purely by appearance edits. 

Second, we enforce a multi-view geometric consistency loss that penalizes discrepancies between Gaussian centers inferred from different views, encouraging them to converge to a shared, view-independent configuration.

\section{DL3DV-Edit-Bench Dataset Details}
\label{sec:DL3DV-edit-bench}

\subsection{Generated Results Summary}
For our DL3DV-Edit-Bench, we select a subset of \textbf{20} static indoor and outdoor scenes from the DL3DV test split and generate a total of \textbf{100} text-driven edits. Each edit is associated with a set of multi-view images and a corresponding natural language instruction. We organize the edits into four categories: (1) \emph{Add} (e.g., add new furniture or decorative objects), (2) \emph{Remove} (e.g., remove existing objects such as chairs or plants), (3) \emph{Modify} (e.g., changing the color or material of an object), and (4) \emph{Global} (e.g., altering the overall lighting or global style of the scene). In our current benchmark, we include approximately \textbf{25} edits per category.

For each scene, we uniformly sample between \textbf{0} and \textbf{20} camera views from the original DL3DV sequence as input views, and generate edited targets for the same set of viewpoints. The input image resolution is fixed to $512\times512$, while we render additional novel-view images at the same resolution to evaluate 3D consistency and generalization.

To reduce annotation noise and ensure that the generated edits are meaningful and feasible, we perform several automatic filtering steps when constructing the benchmark. First, we discard scenes with severe motion blur, very low texture, or large dynamic objects. Second, we remove instructions that are ambiguous, contradictory to the original scene, or that cannot be faithfully applied by the chosen 2D editing model. Finally, we manually spot-check a small subset of edits to verify that the resulting edited images correctly follow the intended instructions and maintain reasonable visual quality.

\subsection{Generated Examples}
\begin{figure*}[t]
    \centering
    \includegraphics[width=0.8\textwidth]{fig/Supp_image_editor.pdf}
    \caption{\textbf{Examples of generated prompts and edited images.}}
    \label{fig:supp_image_editor}
\end{figure*}
To give a more concrete sense of our DL3DV-Edit-Bench, Fig.~\ref{fig:supp_image_editor} shows four representative IP2P examples, each displaying an original input view and the corresponding edited result.
They cover all four edit categories used in our benchmark: \emph{Add} (``Add pictures on the wall'' in an indoor corridor), \emph{Modify} (``Change furniture dark navy'' for a living-room sofa and table), \emph{Remove} (``Remove round table'' in an outdoor plaza), and \emph{Global} (``Make scene cyberpunk neon'' with a strong global style change in a classroom).
These examples illustrate that our edits range from localized object additions/removals to large global appearance changes while remaining reasonably realistic in a single view.

\section{Training Details}
\label{sec:training-details}
% \subsection{Training Datasets \& Setting}
 Our {\ourmethod} model is initialized from the publicly available
$512 \times 512$ NoPoSplat checkpoint, which has been pre-trained on the
RealEstate10K, DL3DV, and ACID datasets. Thanks to this strong initialization, our model
converges significantly faster, and we therefore fine-tune it only on DL3DV
without additional pre-training on RealEstate10K or ACID. 
We use a separate copy of the checkpoint as the frozen LRM for geometry supervision; the {\ourmethod} backbone is initialized from the same checkpoint but is fine-tuned during training.

For DL3DV, we use a training split containing \textbf{10{,}510} video clips,
resulting in approximately \textbf{51.2M} frames in total. At each training
step, we randomly sample one video clip and then draw a set of context views
as inputs together with a separate target view as ground-truth supervision.
Unless otherwise specified, the input and target images are resized to
$512 \times 512$. We employ the AdamW optimizer (Loshchilov \& Hutter, 2018),
setting the initial learning rate for the backbone to $1 \times 10^{-5}$ and
the learning rate for all newly introduced parameters to $1 \times 10^{-4}$.
We use a cosine decay schedule with a linear warm-up phase at the beginning
of training. The model is trained on \textbf{8} NVIDIA RTX~6000 GPUs with a
total batch size of \textbf{8}, \textbf{16000} training steps, which takes roughly \textbf{4} hours to reach convergence. All baseline comparisons in the main paper are obtained from this $512 \times 512$ model fine-tuned on DL3DV.
Unless otherwise stated, all inference timings are measured on a single RTX~6000 GPU, consistent with the main paper.

\section{Quantitative Experiments Supplementary}
\label{sec:quantitative-experiments}
\subsection{Baseline Setup}

\paragraph{EditSplat.}
For EditSplat~\cite{lee2025editsplatmultiviewfusionattentionguided}, we use the official implementation and keep all hyperparameters at their default values.
As required by EditSplat, the method operates on a \emph{pre-trained} 3DGS scene with known camera poses.
For each DL3DV-Edit-Bench scene, we first download the 3DGS model from FCGS ~\cite{chen2025fastfeedforward3dgaussian}, and use this 3DGS as the source scene for all optimization-based baselines.
During editing, EditSplat renders multi-view RGB images (and depth maps) from the source 3DGS, feeds them into InstructPix2Pix (IP2P) with its Multi-view Fusion Guidance (MFG), and then optimizes the 3DGS with Attention-Guided Trimming (AGT) as in the original paper~\cite{lee2025editsplatmultiviewfusionattentionguided}.
In our benchmark, each scene is annotated with a \emph{single} text instruction describing the desired edit, and no additional prompts such as source-scene descriptions or negative prompts are provided.
Therefore, for EditSplat we use this instruction as the only text input to IP2P, and leave all other textual fields to their default values in the released code, so that all methods are conditioned on exactly the same editing instruction.

\paragraph{GaussCtrl.}
GaussCtrl~\cite{gaussctrl} is also an optimization-based method that edits a pre-reconstructed 3DGS scene using a depth-conditioned ControlNet and attention-based latent code alignment.
Similar to EditSplat, GaussCtrl requires a posed 3DGS model as input.
For each DL3DV-Edit-Bench scene we therefore start from the same pre-trained 3DGS used above, render all dataset views and their depth maps at the resolution specified in the official code, and pass them together with camera poses to GaussCtrl.
The original GaussCtrl paper uses \emph{description-like} prompts (a source scene description plus an edited description) as text inputs to ControlNet~\cite{gaussctrl,lee2025editsplatmultiviewfusionattentionguided}.
However, our benchmark only provides a single instruction-type prompt per scene, without any separate source descriptions.
To keep the comparison fair and avoid manually engineering extra text, we use the benchmark’s editing instruction as the \emph{only} text prompt for GaussCtrl, and leave the source-description prompt empty in the official implementation.
All other hyperparameters (number of diffusion steps, guidance scale, reference-view selection, etc.) follow the authors’ default settings.
Under this setup, GaussCtrl, EditSplat, and {\ourmethod} are all driven by the same scene-level editing instruction, while optimization-based baselines additionally require the pre-trained 3DGS and camera poses.

\subsection{User Study}
To further evaluate the perceptual quality of our editing results, we conduct a user study comparing our method with several baselines. We randomly select 10 representative examples and, for each example, render the edited (or generated) views produced by all methods side-by-side in a randomized order. We then recruit 30 volunteers who are not informed of the underlying algorithms. For each example, participants are asked to rate the results from two aspects: (1) \emph{editing faithfulness} (how well the result follows the target edit) and (2) \emph{visual quality} (overall realism and rendering quality). Scores are given on a Likert scale from 1 (worst) to 5 (best). For every metric, we collect all scores across participants and examples, and report the mean and standard deviation for each method in Tab.~\ref{tab:user_study}.

We observe that {\ourmethod} consistently receives the highest scores on both criteria, indicating better semantic alignment and visual realism compared to the baselines.

\begin{table}[t]
\centering
\scriptsize
\caption{\textbf{User scores on editing faithfulness and visual quality}.}
\label{tab:user_study}
\setlength{\tabcolsep}{6pt}

\begin{tabular}{l@{\hskip 8.0mm}c@{\hskip 8.0mm}c}
\toprule
\textbf{Method} & \textbf{Editing Faithfulness~(\(\uparrow\))} &
\textbf{Visual Quality~(\(\uparrow\))} \\
\midrule
EditSplat  & $2.32 \pm 1.03$ & $2.44 \pm 1.31$\\
GaussCtrl & $1.51 \pm 0.63$ & $1.89 \pm 0.62$\\
NoPoSplat  & $3.09 \pm 0.92$ & $2.58 \pm 0.87$\\
{\ourmethod} & $3.49 \pm 0.70$ & $3.45 \pm 0.81$\\
\bottomrule
\vspace{-4mm}
\end{tabular}
\end{table}

\section{Qualitative Experiments Supplementary} %这里用别的人脸数据集的结果
\label{sec:qualitative-experiments}

\subsection{More Results}
As shown in Fig~\ref{fig:supp_results}, here we show six additional results in our qualitative experiments. We compare our method with EditSplat, GaussCtrl, and NoPoSplat. Each example contains 3 views.

\subsection{Results on Other Datasets}

To demonstrate that our model generalizes beyond DL3DV, we additionally conduct qualitative experiments on the classic \textit{Face} and \textit{Bear} scenes from Instruct-NeRF2NeRF~\cite{in2n}, as shown in Fig.~\ref{fig:supp_other_example}.

\section{Failure Cases \& Limitation}
\label{sec:failure-cases}
\begin{figure}[t]  % [t] 顶端
\scriptsize
    \centering
    \hspace{10mm}
    \includegraphics[width=0.8\linewidth]{fig/Supp_failure.pdf}
    \caption{\textbf{Two failure cases.}}
    \label{fig:supp_failure}
    \vspace{-4mm}
\end{figure}

\paragraph{Failure cases.}
As shown in Fig.~\ref{fig:supp_failure}, a common failure mode comes from the 2D editing stage. When the editor (especially InstructPix2Pix~\cite{ip2p}) does not follow the text prompt or severely distorts the input structure, different views may contain mutually inconsistent content or even completely different layouts.
In such cases, our 3D reconstructor cannot reconcile these conflicting observations, leading to strong multi-view inconsistency, objects that only appear in some views, or renders that no longer preserve the original scene geometry.

Another typical failure is also shown in Fig.~\ref{fig:supp_failure}, arising when the target view is very far from the input viewpoints.
Due to GPU memory constraints, our current implementation does not reconstruct a full $360^\circ$ scene and uses a limited number of Gaussian points.
When the camera moves to unobserved regions (e.g., the back side of objects), there may be large areas with sparse or no Gaussian coverage, resulting in visible holes, over-smoothed geometry, or low-opacity ``foggy'' regions in the novel-view renderings.

\paragraph{Limitations.}
First, our method is fundamentally bounded by the capabilities and biases of the upstream 2D editors and the SAM2-based recoloring supervision.
It handles moderate, structure-preserving edits well, but large geometric changes (strong add/remove operations, extreme deformations, or heavy rearrangements) can still produce implausible geometry, inconsistent shadows, or artifacts around occlusion boundaries.

Second, the current design targets static scenes captured by relatively sparse views, with a single text instruction shared across all images.
We do not explicitly model dynamics, very long trajectories, or fine-grained 3D controls (e.g., editing individual objects separately or adjusting their pose in 3D).
Moreover, memory and compute limitations restrict the maximum scene scale and resolution; performance may degrade for very large, highly cluttered scenes or camera paths that deviate significantly from our training and evaluation setup.

\begin{figure*}[t]
    \centering
    \includegraphics[width=\textwidth]{fig/Supp_example_1.pdf}
    \caption{\textbf{More qualitative results.}}
    \label{fig:supp_results}
\end{figure*}

\begin{figure*}[t]
    \ContinuedFloat
    \centering
    \includegraphics[width=\textwidth]{fig/Supp_example_2.pdf}
    \caption[]{\textbf{More qualitative results (continued).}}
\end{figure*}

\begin{figure*}[t]
    \ContinuedFloat
    \centering
    \includegraphics[width=\textwidth]{fig/Supp_example_3.pdf}
    \caption[]{\textbf{More qualitative results (continued).}}
\end{figure*}

\begin{figure*}[t]
    \centering
    \includegraphics[width=\textwidth]{fig/Supp_other_example.pdf}
    \caption[]{\textbf{More qualitative results on other scenes.}}
    \label{fig:supp_other_example}
\end{figure*}

%例子1，图片编辑失败，尤其是ip2p，会出现完全不follow textprompt，或者完全不管图片结构，直接生成完全不一样的图片的情况。这个时候会导致view之间的inconsistency差异非常大，跟场景编辑没有任何关系了。

%例子2，target pose太远，由于显存限制，我们目前的重建还不能做到360度，如果场景中出现target view和输入的视角变化较大，会出现较多空白的地方没有gaussian点。

% % 
% Having the supplementary compiled together with the main paper means that:
% % 
% \begin{itemize}
% \item The supplementary can back-reference sections of the main paper, for example, we can refer to \cref{sec:intro};
% \item The main paper can forward reference sub-sections within the supplementary explicitly (e.g. referring to a particular experiment); 
% \item When submitted to arXiv, the supplementary will already included at the end of the paper.
% \end{itemize}
% % 
% To split the supplementary pages from the main paper, you can use \href{https://support.apple.com/en-ca/guide/preview/prvw11793/mac#:~:text=Delete%20a%20page%20from%20a,or%20choose%20Edit%20%3E%20Delete).}{Preview (on macOS)}, \href{https://www.adobe.com/acrobat/how-to/delete-pages-from-pdf.html#:~:text=Choose%20%E2%80%9CTools%E2%80%9D%20%3E%20%E2%80%9COrganize,or%20pages%20from%20the%20file.}{Adobe Acrobat} (on all OSs), as well as \href{https://superuser.com/questions/517986/is-it-possible-to-delete-some-pages-of-a-pdf-document}{command line tools}.
